# Supplementary material for: Let Trajectories Speak Out the Traffic Bottlenecks
Source: arXiv:2107.12948 source file (2021-07-27)
Supplement: Supplementary file 1 [file sec7-appendix.tex]

\appendix
